# Supplementary material for: A Classification of Connected f -factor Problems inside NP
Source: arXiv:1507.07856 source file (2015-07-28)
Supplement: Supplementary file 1 [file appendix.tex]

\section {Definitions,Procedures and Proofs}
\begin{definition}
\label{kexpansion}
k-expansion of a vertex v is defined as follows.
\begin{enumerate}
\item Construct gadget $G_{k+1}$ by removing a matching of size $\ceil{\frac{k}{2}}-1$ from a complete graph on $k+1$ vertices.
\item Make $v_i$ adjacent to those vertices in $G_{k+1}$ whose degree got reduced by 1.
\end{enumerate}

\subsection{The Reduction Procedure R}
\label{procR}
\end{definition}
\begin{enumerate}
 \item {For even values of $k$, perform $k$-expansion of each vertex $v_i$ in $G$.
}
\item {For odd values of $k$, do the following at each vertex $v_i$ in $G$.
\begin{enumerate}
\item Add vertices $u_1,u_2,\dots,u_{k-2}$.  For $1 \leq j \leq k-2$, make $v_i$ adjacent to all $u_j$.
\item Perform $k$-expansion on each vertex $u_j$.
\end{enumerate}
}
\end{enumerate}
\subsection{3-approximation Algorithm for \MetricMinRTwoCS k}
\label{2MRCS}
\begin{enumerate}
\item Let $OPT_k$ be a solution to the problem of finding minimum weighted $k$-factor in $G$. 
\item {Find the 2-edge connected components in $OPT_k$ using Tarjan's algorithm in \cite{ET75}. Define a partitioning $P'$ as the one induced by the 2-edge connected components of $OPT_k$. Consider the graph $OPT_k/P'$. Consider all those partitions $P'_i \in P'$ that have degree 1 in $OPT_k/P'$. We take the union of these leaf partitions to form the partition $P$. We define $l=|P|$.}
\item We use the 2-approximation 2-TSP for the optimal metric Traveling Salesman Problem  in ~\cite{Shmoys2011}.  %This 2-TSP is of cost at most twice the cost of $T$. %Let the $TSP$ tour $E_{{TSP}}=(v_0,v_1),(v_1,v_2),\dots,(v_{n-1},v_n),(v_n,v_0)$.       
Let $S=v_1,\dots,v_n$ be a cyclic sequence in which the vertices occur in 2-TSP.

%\item  Let $V_{P_i}=v_1^{P_i},v_2^{P_i},\dots,v_{|P_i|}^{P_i}$ be a subsequence of $E_{TSP}$ where each $v_i^{P_i} \in P_i$.
\item For each partition $P_i$ we consider the subgraph $OPT_k[P_i]$ induced by partition $P_i$. Construct a set $V_P$ of $l$ representative vertices one from each $OPT_k[P_i]$. Each representative vertex $v^i$ is part of some cycle $C^{i}$ in $OPT_k[P_i]$. For $1\leq i \leq l$, such a $v^i$ always exists since each $OPT_k[P_i]$ can't be a tree. Let  $S_P=\{v^{1},v^{2},\dots,v^{l}\}$ be a subsequence of $S$ induced by $V_P$. We define a cycle $C_P$ over the set of vertices in $V_P$ as follows. For each pair $v^i,v^{i+1}$ of adjacent vertices in $S_P$ we add the edge $(v_i,v_{i+1})$({\tt /* Note $i+1$ is considered as the value modulo $l$ */}) to  $C_P$.   
%for each $1 \leq i \leq l$, %$v^{i}$ is the first vertex in the sequence $S$ which is an element of $P_i$.  
%Based on this We redefine $E_T$ to be a tour of the form \[E_T=(v_1^{P_1},v_1^{P_2}),(v_1^{P_2},v_1^{P_3}),\dots,(v_1^{P_{l-1}},v_1^{P_{l}}),(v_1^{P_l},v_1^{P_1})\].  
\item Construct a connected spanning subgraph $G'$ of $G$ where $E(G')=E(OPT_k) \cup E(C_P)$. In $G'$ for $1 \leq i \leq l$, $v^{i}$ has degree $k+2$  and every other vertex has degree $k$.   Observe that $G'$ is a multigraph if $l=2$. 
\item For each  $i=1,2,\dots,l$ perform the following sequence of steps:
\begin{enumerate}
\item select a vertex $u^i \in C^i$ such that $(u^i,v^{i}) \in E(G')$. 
\item Remove the edges $(u^i,v^{i})$ and $(v^{i},v^{i+1})$. (addition \textit{modulo} $l$). 
\item Add the edge  $(u^i,v^{i+1})$ to $G'$. 
\end{enumerate}
\end{enumerate}
